# Supplementary material for: Reinforcement Learning from Implicit Neural Feedback for Human-Aligned Robot Control
Source: arXiv:2512.00050 source file (2025-11-18)
Supplement: Supplementary file 1 [file appendices.tex]

\relax
