# Supplementary material for: Reinforcement Learning from Implicit Neural Feedback for Human-Aligned Robot Control
Source: arXiv:2512.00050 source file (2025-11-18)
Supplement: Supplementary file 3 [file appendix_derivation_of_alpha.tex]

This appendix contains no additional material.
